# Supplementary material for: Magnetic cooling for microkelvin nanoelectronics on a cryofree platform
Source: arXiv:1702.06425 ancillary file (2017-02-21)
Supplement: Supplementary file 1 [file supplementary.pdf]

## Supplementary Material

### **Magnetic cooling for microkelvin nanoelectronics on a cryofree platform**

M. Palma,<sup>1, a)</sup> D. Maradan,<sup>1, 2, a)</sup> L. Casparis,<sup>1, 3</sup> T.-M. Liu,<sup>1, 4</sup> F. Froning,<sup>1</sup> and D. M. Zumbühl<sup>1, b)</sup>

<sup>1)</sup>*Department of Physics, University of Basel, Klingelbergstrasse 82, CH-4056 Basel, Switzerland*

<sup>2)</sup>*Physikalisch-Technische Bundesanstalt (PTB), Bundesallee 100, 38116 Braunschweig, Germany*

<sup>3)</sup>*Center for Quantum Devices, Niels Bohr Institute, University of Copenhagen, 2100 Copenhagen, Denmark*

<sup>4)</sup>*Department of Applied Physics, National Pingtung University, Pingtung City, Taiwan*

(Dated: 21 February 2017)

---

<sup>a)</sup>These authors contributed equally to this work.

<sup>b)</sup>dominik.zumbuhl@unibas.ch

## I. SETUP

Figure S1 shows a scheme of the dilution refrigerator from room temperature down to the chip carrier. The measurement leads from the RT flange down to the MC are made by 1.5 m long lossy thermocoaxes, providing an attenuation of 100 dB for frequencies above 300 GHz. Then the leads are connected to microwave filters<sup>1</sup>, which provide an attenuation of 100 dB above 200 MHz and thermalization for the electrons. In addition, we have a second filter stage that consists of two-pole resistor-capacitor filters ( $2 \times [2 \text{ k}\Omega / 680 \text{ pF}]$ ). In order to further improve the thermalization of the measurement leads we use Ag-sinters, where each one of them has dimensions of  $[4 \times 4 \times 20] \text{ mm}^3$  and a surface area of  $4.5 \text{ m}^2$  measured with Brunauer-Emmett-Teller (BET) surface area analysis<sup>2</sup>. Doubling the number of sinters per lead compared to the previous setup<sup>3</sup> allows us to reach a lower precooling temperature in less time. As discussed in the main text we further doubled the diameter of the annealed high-purity 5N (99.999%) Ag wire ( $\varnothing = 2.54 \text{ mm}$ ) coming out of the MC, to enhance the cooling. Each Ag wire is spot-welded to a Cu plate, resulting in the parallel network of 16 nuclear refrigerators. In addition, we doubled the amount of Cu per plate by spot-welding 2 half plates together. Each half plate has dimensions of  $[34 \times 1.7 \times 120] \text{ mm}^3$ , corresponding to 1 mol. In order to shield the 16 NRs, we use radiation shields which are attached to the still flange (around 650 mK) and mixing chamber flange (below 7 mK). As indicated below the dashed red line in Fig. S1, we design a sample holder with 15 commercial pins for transport experiments. The sample holder is made of sapphire, which is a low heat release material, has a hole in the center to allow an annealed Ag wire to pass through and cool the metallic plane of the plug-in sapphire chip carrier. Using plug-in pins is practical to exchange samples, but the plug-in mechanism might cause strain, which is a possible source of heat release. The chip carrier is enclosed in a Faraday cage that functions as sample shield. The sample holder and the chip carrier were not installed at the time of the measurements reported in the main text and will be only considered in the last paragraphs of the supplementary material.

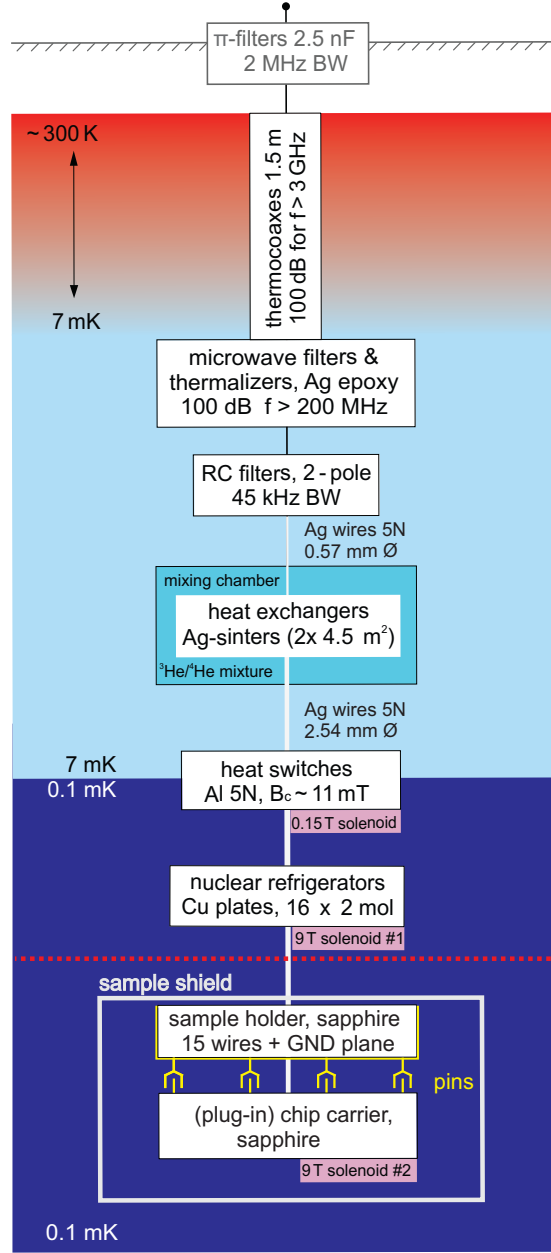

FIG. S1. Scheme of the dilution unit together with NRs. Compared to Ref. [3] we doubled the number of sinters per lead, the diameter of the silver wires and the amount of Cu per plate. Below the dashed red line, the socket design for future transport experiments is illustrated. The abbreviations in the figure are bandwidth (BW), critical magnetic field ( $B_c$ ) and the electrical ground (GND).

## II. HIGH PERFORMANCE SYSTEM

Figure S2(a) shows the temperature recorded with the MFFT (red squares) and CMN (blue line) for a typical precooling at 9 T. The temperature of both sensors decreases from 38 mK down to 9.8 mK in 85 hours. However, in 30 hours we reach a  $T_s$  of 13 mK, which could have been already used to perform an AND. As shown in Fig. S2(a) the cooling in the first 15 hours is less efficient than the theory<sup>4</sup> predicts, where at later time the experimental data follows the theory (depicted as dashed line) more closely. In order to perform electronic transport experiments, it is important to evaluate the hold time (below 1 mK). Therefore, in Fig. S2(b) we plot again the warm up curve for two final fields of 80 mT and 200 mT, measured with the MFFT. We obtain hold times of 50 hours for 80 mT and 80 hours for 200 mT, owing to the low static heat leak.

In the main text we discuss the static heat leak measured with the MFFT for various  $B$ -fields (inset of Fig.3(b)). In Fig. S3, we present the same measurements for the CMN and LCMN thermometers. The static heat leak  $\dot{Q}$  is  $B$ -field independent below 1 T for both sensors, as observed for the MFFT. In addition, the static heat leak for the LCMN ( $\dot{Q}=3$  nW/mol) and the CMN ( $\dot{Q}=2.2$  nW/mol) thermometer is higher compared to the MFFT, possibly because of an increased amount of heat release of the thermometers.

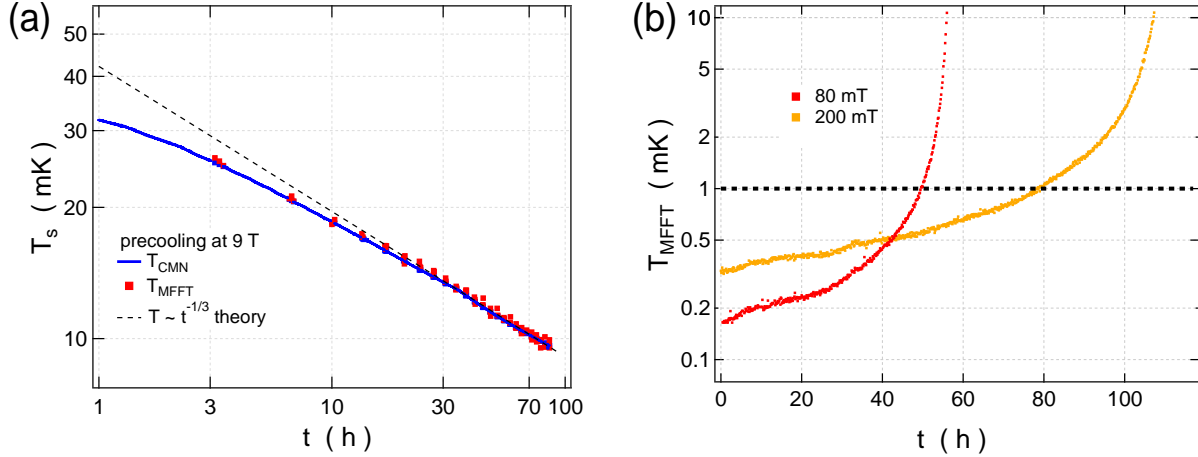

FIG. S2. (a) shows the temperature of the CMN thermometer and MFFT as function of the time during the precooling at 9 T. The dashed line indicates the behavior of the precooling temperature predicted from the theory<sup>4</sup>. (b)  $T_{\text{MFFT}}$  versus time for warm ups at 80 mT and 200 mT. The dashed line points out the hold time below 1 mK, which is important for transport experiments.

### III. WARM UP

As shown in Fig. S4, the inverse of  $T_s$  measured with CMN and LCMN thermometers is fitted with Eq. (2) of the main text. The extrapolated Cu electron temperature  $T_{\text{ex}}$  is close to the value obtained from the fit of the MFFT data in Fig. 3(a) of the main text. In Fig. S4(b) we show that the thermal model, presented in Eq. (3) of the main text, reproduces well the experimental data for the CMN and the LCMN thermometer. The CMN thermometer is still cooling in the first hours of the warm up in contrast to the LCMN thermometer, possibly due to the higher heat capacity of the CMN<sup>5</sup> compared to the LCMN. From the fit of Eq. (3), we extract a sensor heat leak  $\dot{Q}_s$  around 10-20 % of  $\dot{Q}$  for both thermometers, which is an indication for a small heat leak coming from the thermometer, such values are similar to the  $\dot{Q}_s$  extracted for the MFFT. The higher heat leak of LCMN and CMN could arise from the screw press contact resistance of about  $100 \mu\Omega$  between the thermometers and the connection to the NRs. For the MFFT we take into account only the resistance of the Ag-wire and the weld-joint between Ag wire and the Cu plate, which gives a total resistance of about  $1 \mu\Omega$ .

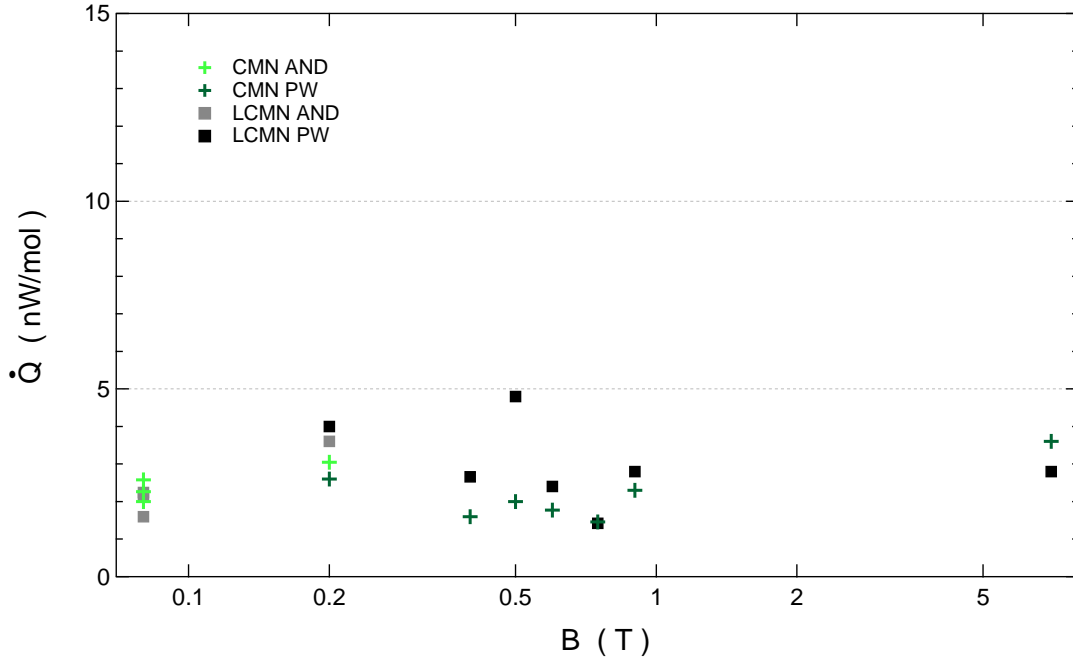

FIG. S3.  $\dot{Q}$  at various  $B$ -fields measured with CMN and LCMN thermometers. The static heat leaks  $\dot{Q}$  are extracted with PW and AND methods introduced in the main text.

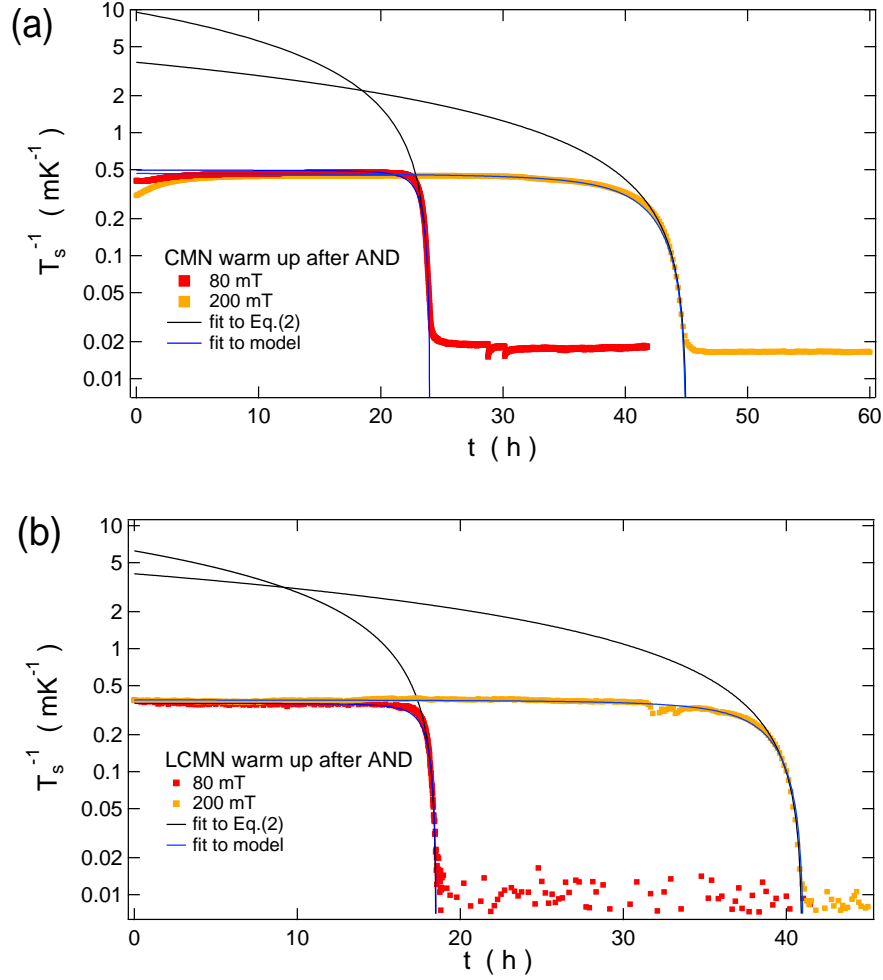

FIG. S4. (a) inverse of  $T_s$  measured with the CMN thermometer versus time during the warm up at 80 mT and 200 mT. The warm up curves are plotted in semi-logarithmic scale, for this reason the lines appear as curves. The fit to Eq. (2) gives an extrapolated Cu electron temperature  $T_{\text{ex}} = 105/268 \mu\text{K}$  and static heat leak  $\dot{Q} = 2.6/3.1 \text{ nW/mol}$  for 80/200 mT, respectively. The solid blue line shows the heat flow model with  $\dot{Q}_s = 9/10 \%$  of  $\dot{Q}$ . (b) shows the same warm up curves for the LCMN thermometer. From the fit to Eq. (2) we extract  $T_{\text{ex}} = 160/246 \mu\text{K}$  and  $\dot{Q} = 2.1/3.6 \text{ nW/mol}$  for 80/200 mT, respectively. The heat flow equation reveals  $\dot{Q}_s = 11/22 \%$  of  $\dot{Q}$  for 80/200 mT, respectively.

#### IV. SOCKET

So far we presented data only referring to NRs without any socket and carrier structure. The introduction of these additional parts might affect the performance of the NRs due to the heat load of the additional material introduced. Therefore we compared the static heat leak measured with MFFT for two different sockets. First, we used a Ag-epoxy socket with a geometry as discussed in the setup paragraph, but with an additional microwave-filter incorporated in the socket. Ag-epoxy is a conductive glue, which enhances the cooling of the chip through the substrate but, however, it is a material with heat release due to structural relaxation of low energy excitations<sup>4</sup>. In Figure S5, the heat leak for the Ag-epoxy socket (black triangles) is measured for various  $B$ -fields. We obtain an average  $\dot{Q}$  between 3 and 4 nW/mol, independent of the  $B$ -field. By comparing this data to the inset of Fig. 3(b), where no socket was installed, the heat release of the Ag-epoxy socket is a factor of 2 higher. In order to reduce the heat release we replace the Ag-epoxy by sapphire, that due to the crystalline structure is supposed to have low heat release. The measured heat leak is around 2 nW/mol and  $B$  independent below 1 T. The heat leak for sapphire socket is in general lower compared to Ag-epoxy socket but higher than with no socket.

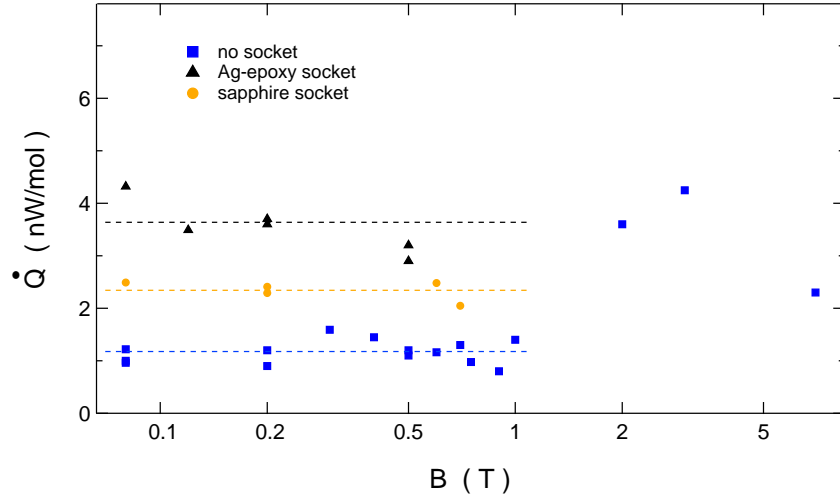

FIG. S5. The static heat leak  $\dot{Q}$  measured with MFFT for various magnetic fields and for three different socket designs: no socket, Ag-epoxy socket and sapphire socket. The dashed lines are guides for the eyes

## V. GRADIOMETER DESIGN

Here, we discuss the improvements that we have done to the design of the noise thermometer. In the first design the thermometer was in direct contact with the superconducting shields, which could introduce additional heat leaks onto the thermometer. Therefore in the second design, we mounted the thermometer contact-less. We introduced a shield holder, which thermalizes the superconducting shields to the support structure without touching the thermometer. Figure S6 shows the data already presented in Fig. 4 of the main text for direct contact (black triangles) and contact-less mounting (blue squares and orange circles) of the thermometer. For the design with direct contact we observe a deviation of the measured temperature from the extrapolated temperature already below 2 mK, which leads to a saturation of  $T_{\text{MFFT}}$  at  $740 \mu\text{K}$ . In contrast, for the contact-less mounting of the thermometer  $T_{\text{MFFT}}$  agrees well with  $T_{\text{e,Cu}}$  down to the lowest temperatures. Note that for the contact-less mounting of the thermometer we used two different socket configurations: sapphire socket and no socket. Despite their different heat leaks the temperature reading of the MFFT is the same. As result the contact-less mounting of the noise thermometer indeed reduces the heat leaks onto the noise source, leading to a lower temperature reading of the MFFT.

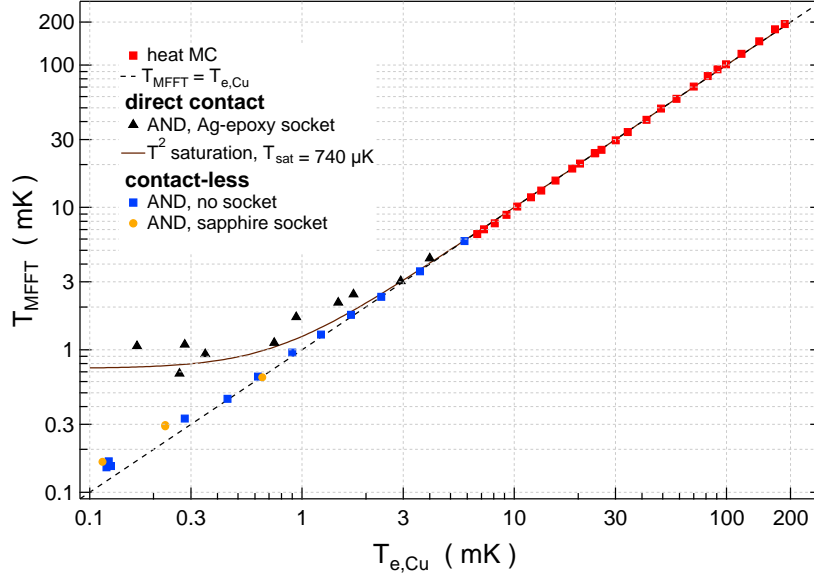

FIG. S6. Temperature measured by MFFT versus the temperature of the nuclear stage  $T_{\text{Cu}}$  with  $T_{\text{Cu}}$  extracted as in Fig. 4 of the main text. We compare two different gradiometer designs: old design with Ag-epoxy socket and improved design realized for no socket and sapphire socket.

## REFERENCES

- <sup>1</sup>C. P. Scheller, S. Heizmann, K. Bedner, D. Giss, M. Meschke, D. M. Zumbühl, J. D. Zimmerman, and A. C. Gossard, “Silver-epoxy microwave filters and thermalizers for millikelvin experiments,” *Appl. Phys. Lett.* **104**, 211106 (2014).
- <sup>2</sup>S. Brunauer, P. H. Emmett, and E. Teller, “Adsorption of gases in multimolecular layers,” *J. Am. Chem. Soc.* **60**, 309–319 (1938).
- <sup>3</sup>A. V. Feshchenko, L. Casparis, I. M. Khaymovich, D. Maradan, O.-P. Saira, M. Palma, M. Meschke, J. P. Pekola, and D. M. Zumbühl, “Tunnel-junction thermometry down to millikelvin temperatures,” *Phys. Rev. Appl.* **4**, 034001 (2015).
- <sup>4</sup>F. Pobell, *Matter and Methods at Low Temperatures* (Springer, Berlin, 2007).
- <sup>5</sup>B. M. Abraham, O. Brandt, Y. Eckstein, J. B. Ketterson, M. Kuchnir, and P. Roach, “Heat capacity of diluted cerium magnesium nitrate and its potential for the production of very low temperatures,” *Phys. Rev.* **187**, 273–275 (1969).
